# Supplementary material for: Quantum dot opto-mechanics in a fully self-assembled nanowire
Source: arXiv:1405.2821 source file (2014-05-12)
Supplement: Supplementary file 1 [file SuppInfo.pdf]

# SUPPORTING INFORMATION

# Quantum dot opto-mechanics in a fully self-assembled nanowire

M. Montinaro,[1] G. Wüst,[1] M. Munsch,[1] Y. Fontana,[2] E. Russo-Averchi,[2] M. Heiss,[2] A. Fontcuberta i Morral,[2] R. J. Warburton,[1] and M. Poggio[1, a)]

[1)] *Department of Physics, University of Basel, Klingelbergstrasse 82, 4056 Basel - Switzerland*

[2)] *Laboratoire des Matériaux Semiconducteurs, École Polytechnique Fédérale de Lausanne, 1015 Lausanne - Switzerland*

## I. MECHANICAL PROPERTIES OF THE NANOWIRE

We calculate the lowest order flexural vibrations and the induced dynamic strain of the nanowire (NW) using a finite element model (FEM) of the experimental system. We approximate the NW structure as an isotropic hexagonal prism of AlGaAs, with a density given by the average of the densities of the different GaAs and AlGaAs layers, each weighted according to its thickness (see main text). The dimensions of the NW as well as its length that is tightly glued to the Si substrate on a lateral facet are measured by scanning electron microscopy (SEM).

The FEM provides the eigenfrequencies of the NW flexural vibrations and the corresponding mode shapes. While a symmetric clamping of the NW would result in doubly degenerate vibration modes, the asymmetry of the actual clamping geometry, i.e. with only one lateral facet in contact with the substrate, splits each mode into a doublet of flexural vibrations oriented either parallel or perpendicular to the Si surface, with the former having the lower eigenfrequency. Figure 1 shows the mode shape of the lowest 4 non-degenerate vibrations. The spectral separation between two non-degenerate modes in each doublet depends, aside from the nature of the clamping, on the symmetry of the NW geometry: a dilatation of the hexagonal cross-section by only 1% along one axis is enough to invert the spectral positions of the two modes.

As discussed in the main text, in this experiment we focus our attention on the lowest order perpendicular mode. This orientation is preferentially driven by the piezoelectric transducer attached to the sample, is more easily detected by the interferometer, and driving higher order modes requires higher mechanical excitation power or a more sensitive displacement detection. The calculation of the normalized displacement of the favored flexural mode $u_\perp(\boldsymbol{r})$ as a function of the position $\boldsymbol{r}$ allows us to determine the corresponding motional mass $m$ at the NW free-end, according to the definition:

$$m \equiv \int_V \rho \left|u_\perp(\boldsymbol{r})\right|^2 \, d\boldsymbol{r}, \tag{1}$$

where the integral is calculated over the entire NW volume $V$ and $\rho$ is the NW density, which in our model does not depend on $\boldsymbol{r}$. The result is $m = (3.5 \pm 0.7) \times 10^{-15}$ kg, where the error is dominated by the measurement imprecision of the NW thickness.

The flexural vibrations produce a time-varying material strain in the NW, which translates into a uniaxial stress along the NW growth direction ($[1\,\bar{1}\,1]$ in crystallographic notation). This oscillating material strain is responsible for the modulation of the QD emission energy, therefore it is important to evaluate its strength and its spatial distribution. For this purpose, it is necessary to determine the values of the Young's modulus $E_\mathrm{Y}$ and of the Poisson's ratio $\nu$, which fully characterize the elastic properties of isotropic materials[1].

To our knowledge, for a GaAs/AlGaAs nanostructure grown along $\langle 1\,1\,1 \rangle$, $E_\mathrm{Y}$ has not yet been measured. The only reference[2] is the value along this axis measured for bulk GaAs (141.2 GPa). For this reason, we initially set $E_\mathrm{Y}$ as a free parameter in our FEM, while calculating the NW eigenfrequencies. We then tune $E_\mathrm{Y}$ in the FEM until the calculated resonance frequency of the lowest perpendicular mode matches our experimentally measured value of 795 kHz. The corresponding Young's modulus is $E_\mathrm{Y} = 153$ GPa, which is 8% larger than the aforementioned value measured for bulk GaAs. Possible reasons for this increase of the stiffness of our NW reside in its finite size and in its core/shell structure, which introduces an additional intrinsic material strain.

The Poisson's ratio expresses the relative strength of the strain tensor components. By setting an $xyz$ reference system with $\hat{z}$ oriented along the NW growth direction, the strain tensor in our case assumes the following diagonal form:

$$\varepsilon_{ij} = \begin{bmatrix} \varepsilon_\perp & 0 & 0 \\ 0 & \varepsilon_\perp & 0 \\ 0 & 0 & \varepsilon_\parallel \end{bmatrix}. \tag{2}$$

In this reference system, the Poisson's ratio is defined as follows:

$$\nu = -\frac{\varepsilon_\perp}{\varepsilon_\parallel}. \tag{3}$$

Signorello *et al.*[3] have recently measured $\nu$ for Zinc-Blende GaAs/AlGaAs core/shell NWs grown along $\langle 1\,1\,1 \rangle$, as in our case, at a temperature of 100 K (see Table I).

Once these fundamental parameters have been inserted into our FEM, we compute the strain distribution along

a) Electronic mail: martino.poggio@unibas.ch

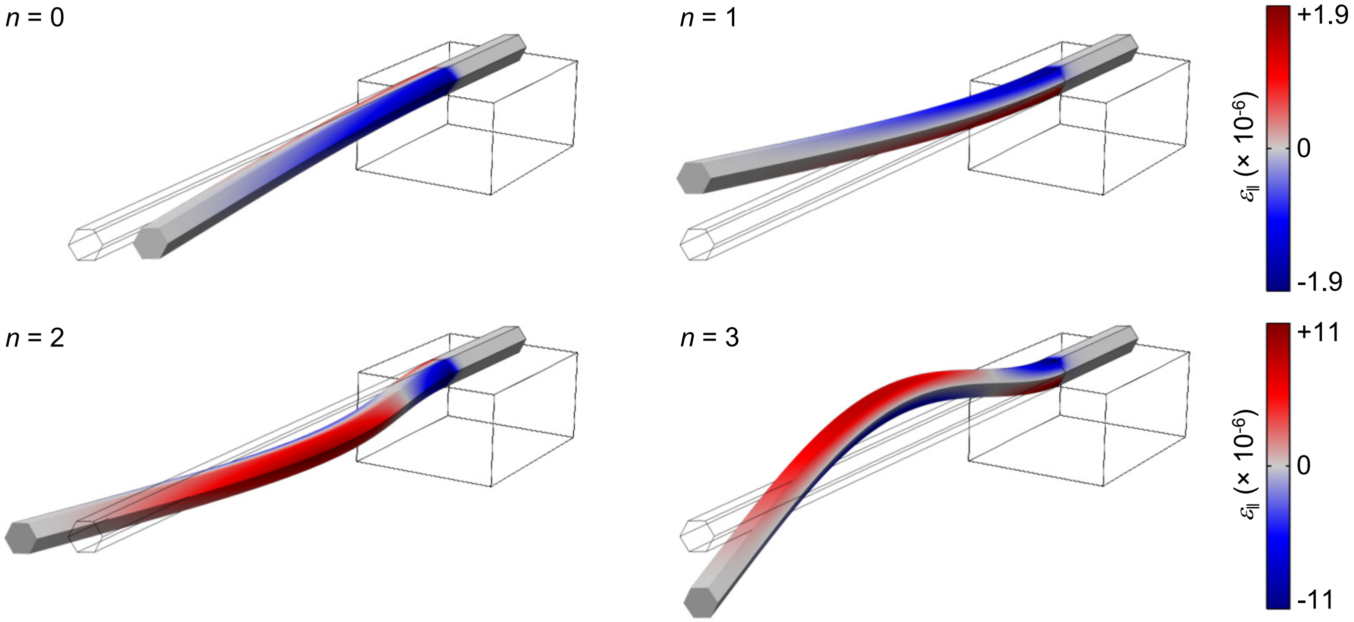


Figure 1. FEM of the NW mechanical properties. Each inset shows the mode shape of the lowest 4 non-degenerate vibrations, $n$ being the mode index. The color scale is proportional to the component $\varepsilon_{\parallel}$ of the material strain in the NW, for a 1-nm displacement of its free end.

the NW structure. Fig. 1 shows in color scale $\varepsilon_{\parallel}$ for the lowest 4 non-degenerate flexural vibrations, for a NW free-end displacement of 1 nm. The doublet described by the mode indices $n = 2$ and 3 has a mode shape characterized by a node near the free end of the NW, resulting in a maximum strain at the clamped end that is a factor 6 larger than the value of the lower index doublet. As confirmed by the FEM analysis, flexural modes of even higher index result in a further increase of the strain at the clamped end. Improvements in the excitation and detection of these higher modes should provide an opto-mechanical coupling parameter increased as the strain. However, the coupling rate $\lambda$ defined in the main text also depends on the NW's zero-point motion $x_{\mathrm{ZPF}} = \sqrt{\hbar/\left(2m_n\Omega_n\right)}$. While the mode motional mass $m_n$ depends in our geometry very weakly on $n$, the mode resonance frequency $\Omega_n$ increases with $n$, by a factor 6 for the second order doublet with respect to the first one. This dependence implies an increase of $\lambda$ by a factor 2 (or bigger) by driving the NW at its second order (or higher) doublet.

| Parameter | Value | Unit |
|---|---|---|
| $\nu$ | $0.16 \pm 0.04$ | |
| $a$ | $-8.6 \pm 0.7$ | eV |
| $d$ | $-5.2 \pm 0.7$ | eV |

Table I. Electro-mechanical material parameters. The values have been measured for Zinc-Blende GaAs/AlGaAs core/shell NWs grown along $\langle 1\,1\,1 \rangle$, at a temperature of 100 K. Taken from Ref. 3.

## II. EFFECT OF STRAIN ON THE EXCITON TRANSITION ENERGY

The modulation of the exciton transition energy is due to the strain dependence of the QD band structure. The shear and hydrostatic components of the strain both contribute to this opto-mechanical coupling, with a weight given by their respective deformation potential, conventionally indicated as $a$ for the hydrostatic deformation and $d$ for the shearing induced by a stress along $\langle 1\,1\,1 \rangle$[4,5]. The aforementioned work of Signorello *et al.*[3] has obtained these deformation potentials for NWs similar to ours (but without embedded QDs); the measured values are reported in Table I.

The brightest exciton transition in our QDs concerns the conduction and the heavy-hole bands, each responding in a different way to the applied strain. The variation of the energy gap between these bands ($\Delta E^{\text{C-HH}}$) under mechanical excitation can be connected to the strain component $\varepsilon_{\parallel}$ through the following model[4]:

$$\Delta E^{\text{C-HH}} = \left[ (1 - 2\nu)\, a + \frac{1}{\sqrt{3}} (1 + \nu)\, d \right] \varepsilon_{\parallel}. \tag{4}$$

From the FEM of the NW, we extract the profile of $\varepsilon_{\parallel}$ along $\hat{z}$ corresponding to the lowest order perpendicular mode, for a given displacement of the NW free end. The graph in Fig. 2 shows such a plot for $\varepsilon_{\parallel}$ at 10 nm below the NW surface, a distance where the QDs best coupled to strain are located. The red spot, in particular, marks the position where the QDs analyzed in the main text are placed, $2.0 \pm 0.3\,\mu$m away from the clamped

edge of the NW. Inserting the value of $\varepsilon_{\parallel}$ at the QD position into the Eq. 4, we obtain a displacement-dependent energy shift of $13 \pm 2\,\mu$eV/nm. Though this estimation does not take into account the detailed QD band structure, the value we have found is close to our experimental result ($9.9 \pm 0.7\,\mu$eV/nm), therefore confirming the strain-dependence of the band structure as the dominant coupling mechanism.

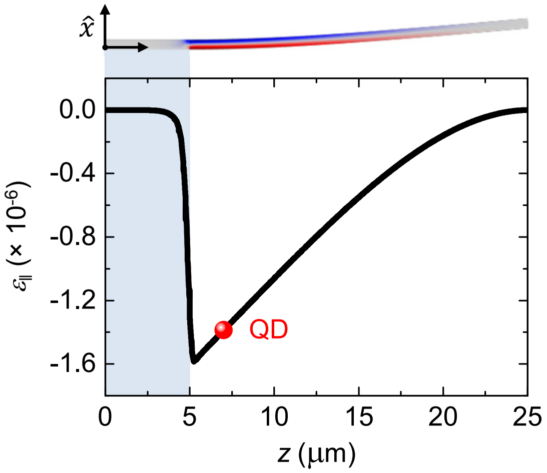


Figure 2. Strain profile along $\hat{z}$. The strain component $\varepsilon_{\parallel}$ is plotted for the NW free-end displaced through $u_{\perp}$ by 1 nm along $\hat{x}$. The shaded area from $z = 0$ to $z = 5\,\mu$m marks the region of the NW which is clamped to the substrate. The red spot at $z = 2.0 \pm 0.3\,\mu$m from the edge of the clamped region marks the position where the QDs analyzed in the main text are located. The upper inset shows the mode shape in consideration, with the strain amplitude in color scale as in Fig. 1.

## III. INTERFEROMETRIC DISPLACEMENT DETECTION

We use a 780-nm laser interferometer to detect the displacement of the NW free-end. Due to the low finesse of our cavity, the interferometer fringe as a function of the cavity length or of the laser wavelength is well approximated by a sinusoid. The NW oscillation modulates the interferometer response in a small range around the fringe average, where the response becomes linear. We stabilize the interferometer in this linear regime, by controlling the laser wavelength via a PID feedback loop.

The cavity free spectral range measures $(2.6 \pm 0.1) \times 10^{-13}$ m, from which we derive a cavity length of $118 \pm 5$ cm. Measurements of the NW displacement are calibrated by an accurate determination of the laser wavelength. In order to double-check this calibration, we measure the displacement amplitude $A_{\rm osc}$ of the positioning stage along $\hat{x}$, while the stage is driven by a low-frequency oscillation (117 Hz). As shown in Fig. 3, the measurement is repeated for several drive voltages in order to extract, through a linear fit, a conversion factor for the piezoelectric positioning stage equal to $11.6 \pm 0.1$ nm/V. The entire procedure is repeated with the interferometer aligned to a variety of different positions on the $yz$ plane, including the position of the NW free end. The values measured using our interferometer are close to the specifications of the positioning stage, which provide a rough conversion factor of 8 nm/V.

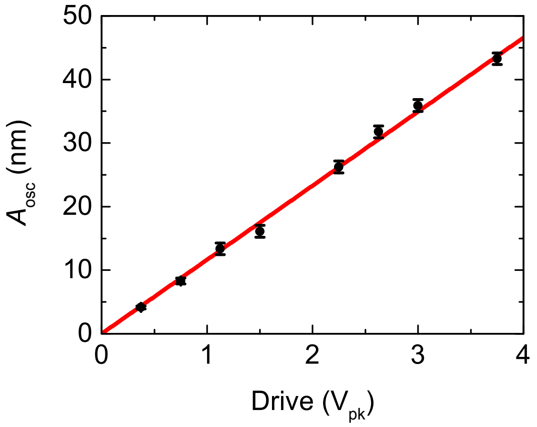


Figure 3. Interferometer test. Amplitude of the positioning stage displacement oscillation at 117 Hz as a function of the amplitude of the drive voltage, measured at a temperature of 4.2 K. The error bars correspond to the peak-to-peak amplitude of the interferometric noise. The red line is a linear fit, from which we extract a conversion factor of $11.6 \pm 0.1$ nm/V.

## REFERENCES


[1] A. N. Cleland, *Foundations of nanomechanics* (Springer ed., 2003).

[2] W. A. Brantley, Journal of Applied Physics **44**, 534 (1973).

[3] G. Signorello, S. Karg, M. T. Björk, B. Gotsmann, and H. Riel, Nano Letters **13**, 917 (2013).

[4] M. Chandrasekhar and F. H. Pollak, Physical Review B **15**, 2127 (1977).

[5] C. G. Van de Walle, Physical Review B **39**, 1871 (1989).
